# Supplementary material for: Uncertainty-Guided Chain-of-Thought for Code Generation with LLMs
Source: arXiv:2503.15341 source file (2025-03-19)
Supplement: Supplementary file 1 [file appendix.tex]

\begin{figure*}
\centering
\begin{AcademicBox} [Case Study]
    \small
    \vspace{1mm}
\noindent Input Requirement:\\ 
\noindent from typing import List\\ 
    \indent\qquad def maximum\_num\_of\_blocks(area: List[int], mass: List[int]) -> int:\\
    \indent\qquad """When playing with building blocks, we usually place small and light building blocks on top of larger and heavier building blocks. Given the mass and area of the building blocks, please calculate the maximum number of building blocks that can be stacked?\\
    \indent\qquad height.length == weight.length <= 10000\\
    \indent\qquad >>> maximum\_num\_of\_blocks([65,70,56,75,60,68], \indent\qquad[100,150,90,190,95,110])\\
    \indent\qquad6\\
    \indent\qquad >>> maximum\_num\_of\_blocks([6, 7, 8], [2, 1, 6])\\
    \indent\qquad2\\
    \indent\qquad"""\\
    \\
\textbf{Baseline Output (Greedy Search):}\\
\vspace{-10pt} 
\begin{minted}[breaklines,fontsize=\small]{python}
    # sort by area
    area_mass = sorted(zip(area, mass))
    # sort by mass
    mass_area = sorted(zip(mass, area))

    # dp[i] = max number of blocks that can be stacked with area[i]
    dp = [1] * len(area)
    for i in range(1, len(area)):
        for j in range(i):
            if area_mass[i][0] > area_mass[j][0] and mass_area[i][0] > mass_area[j][0]:
                dp[i] = max(dp[i], dp[j] + 1)
    return max(dp)
\end{minted}

\textbf{Self-Planning Output:}\\
\vspace{-10pt} 
\begin{minted}[breaklines,fontsize=\small]{python}
    # Let's think step by step
    # 1. Create a list "lis" with the area and mass of the building blocks.
    # 2. Sort the list "lis" in descending order.
    # 3. Initialize a variable "count" with 0.
    # 4. Iterate over the elements of the list "lis".
    # 5. If the area of the building block is greater than the area of the previous building block, add 1 to the variable "count".
    # 6. Return the variable "count".
    # Write your code here
    lis = list(zip(area, mass))
    lis.sort(reverse=True)
    count = 0
    for i in range(len(lis)):
        if i == 0:
            count += 1
        elif lis[i][0] > lis[i-1][0]:
            count += 1
    return count
\end{minted}

\textbf{UnCerT-CoT Output:}\\
\vspace{-10pt} 
\begin{minted}[breaklines,fontsize=\small]{python}
    area_mass = sorted(zip(area, mass))
    dp = {}
    for i in area_mass:
        dp[i] = 1
        for j in dp:
            if i[0] > j[0] and i[1] > j[1]:
                dp[i] = max(dp[i], dp[j] + 1)
    return max(dp.values())
\end{minted}

%edit end
\end{AcademicBox}
\label{fig: few shot}
\end{figure*}
